# Supplementary material for: Escaping Data Scarcity for High-Resolution Heterogeneous Face Hallucination
Source: arXiv:2203.16669 source file (2022-03-30)
Supplement: Supplementary file 1 [file supplementary_table2.tex]

\begin{figure*}[htbp]
        \setlength{\tabcolsep}{1.8pt}
        \centering
        {\small
            \begin{tabular}{c c c c c c c}
                \includegraphics[width=0.13\textwidth]{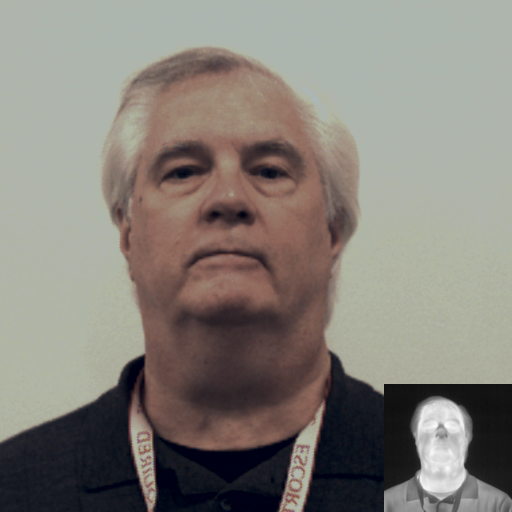}&
                \includegraphics[width=0.13\textwidth]{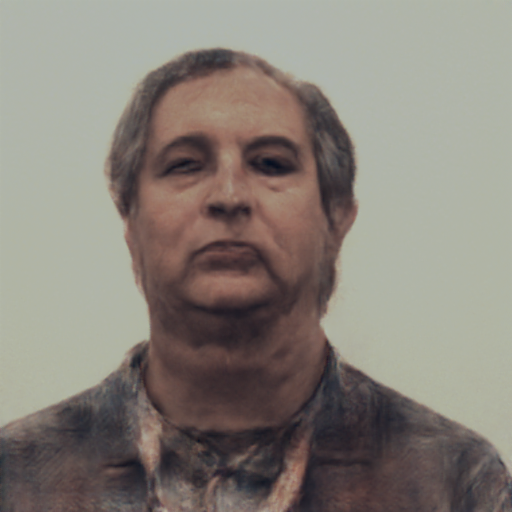}&
                \includegraphics[width=0.13\textwidth]{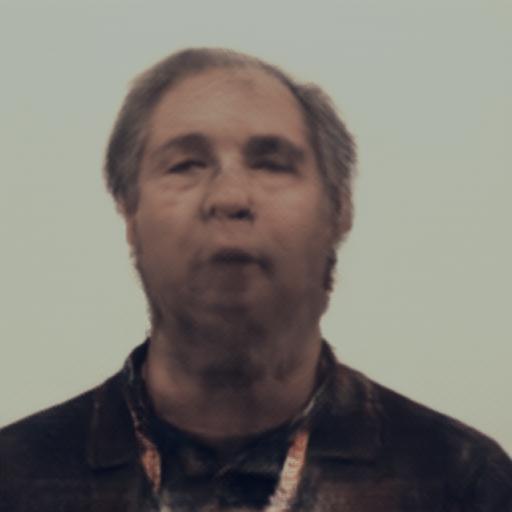}&
                \includegraphics[width=0.13\textwidth]{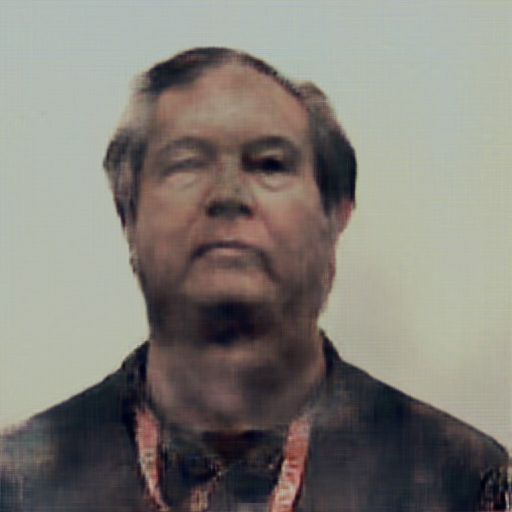}&
                \includegraphics[width=0.13\textwidth]{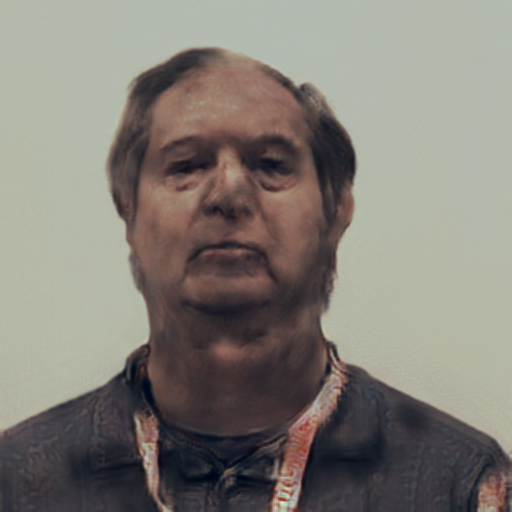}&
                \includegraphics[width=0.13\textwidth]{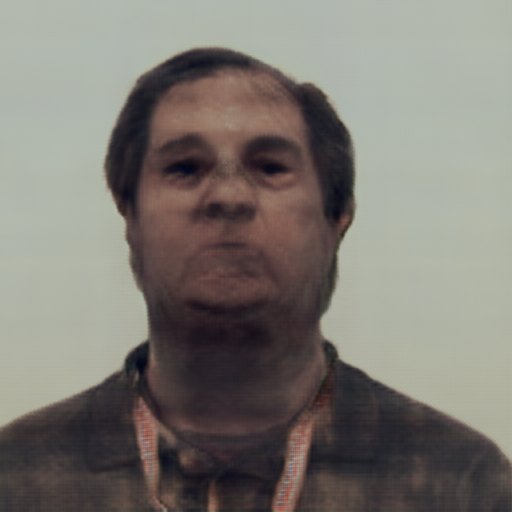}&
                \includegraphics[width=0.13\textwidth]{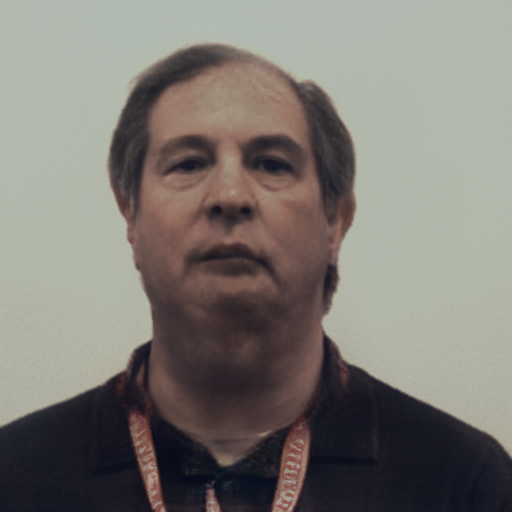}
                \tabularnewline
                \includegraphics[width=0.13\textwidth]{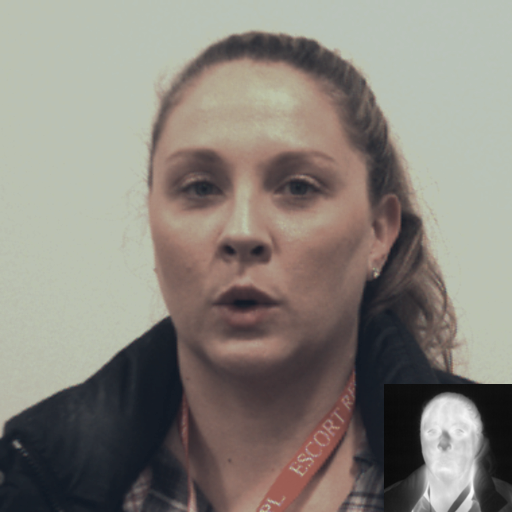}&
                \includegraphics[width=0.13\textwidth]{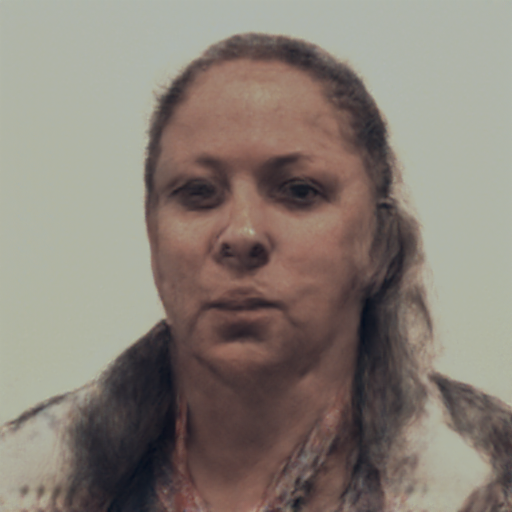}&
                \includegraphics[width=0.13\textwidth]{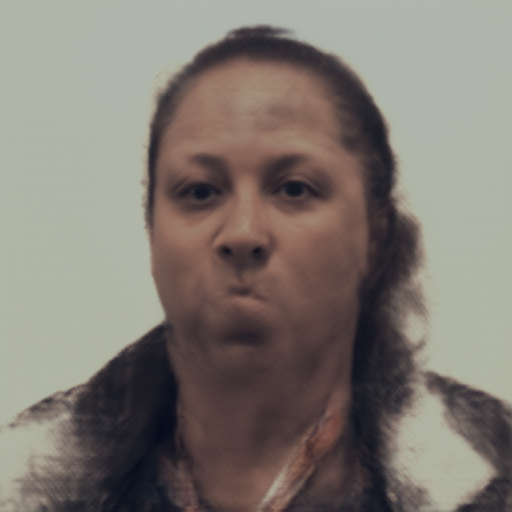}&
                \includegraphics[width=0.13\textwidth]{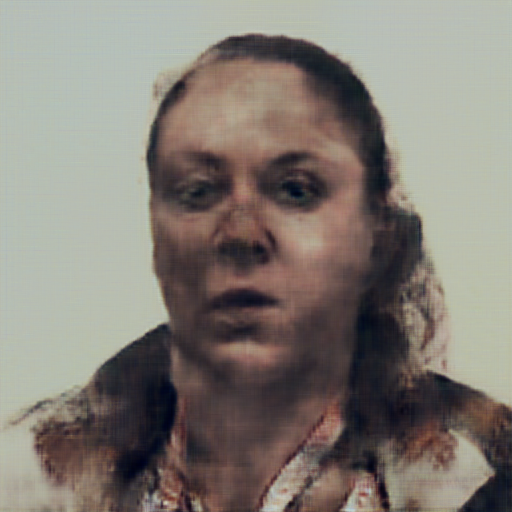}&
                \includegraphics[width=0.13\textwidth]{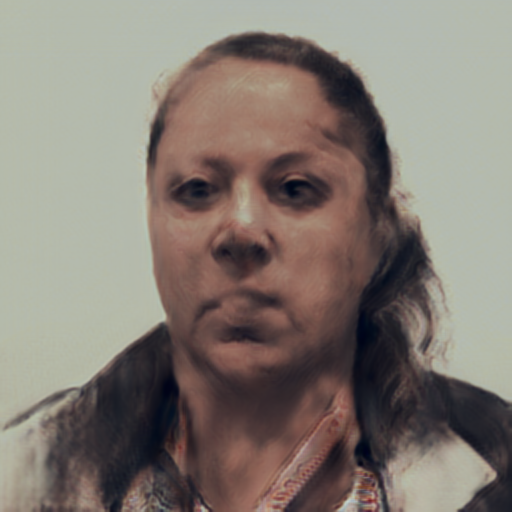}&
                \includegraphics[width=0.13\textwidth]{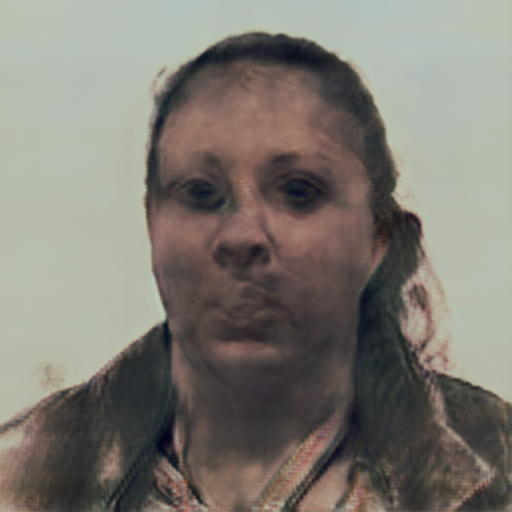}&
                \includegraphics[width=0.13\textwidth]{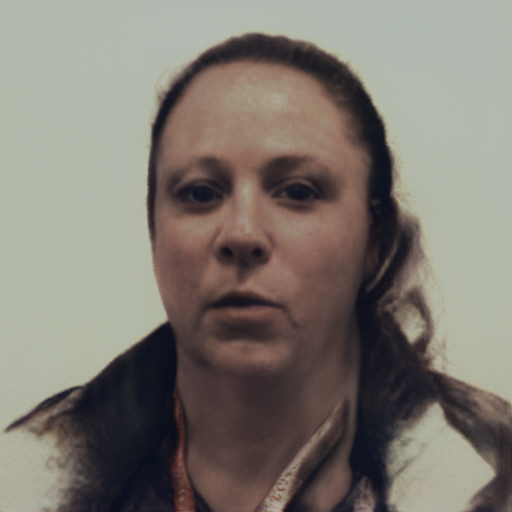}
                \tabularnewline
                \includegraphics[width=0.13\textwidth]{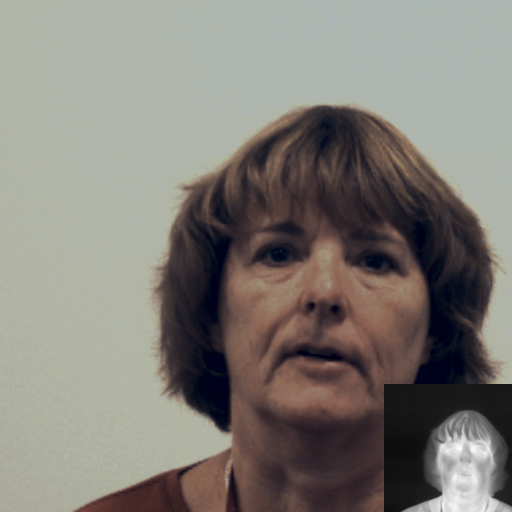}&
                \includegraphics[width=0.13\textwidth]{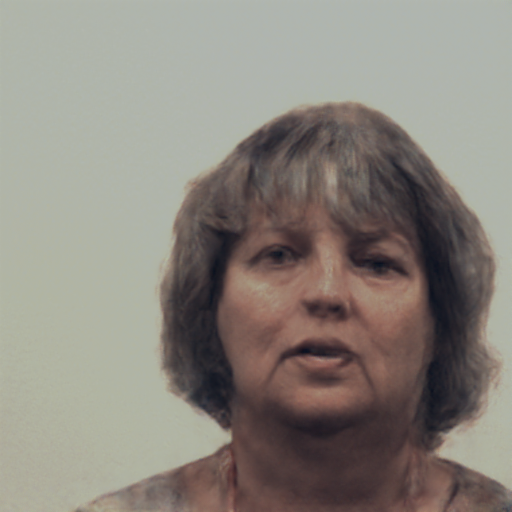}&
                \includegraphics[width=0.13\textwidth]{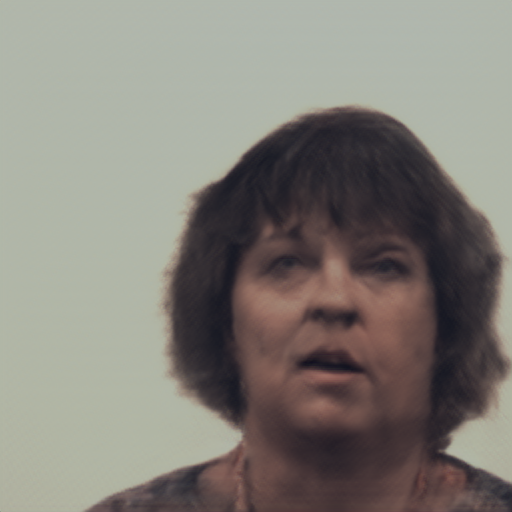}&
                \includegraphics[width=0.13\textwidth]{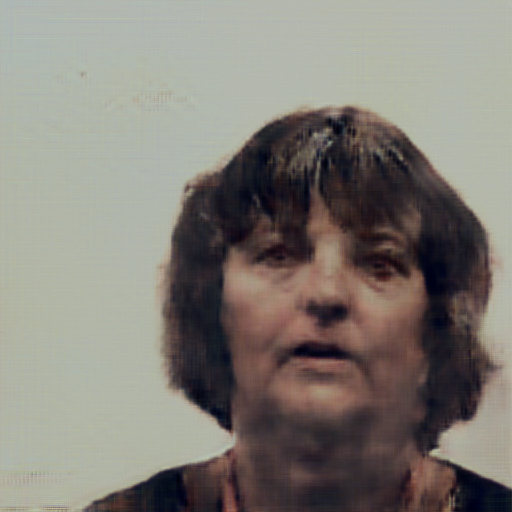}&
                \includegraphics[width=0.13\textwidth]{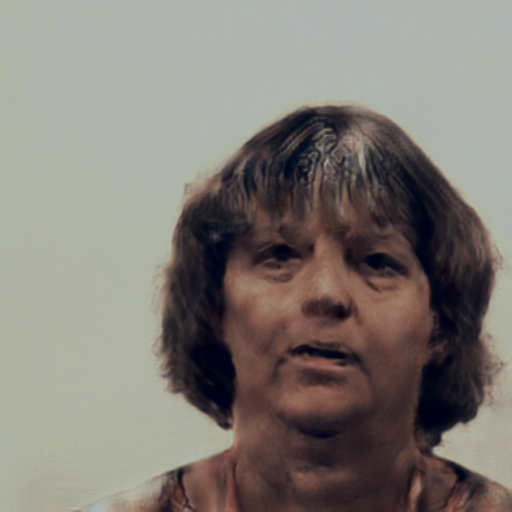}&
                \includegraphics[width=0.13\textwidth]{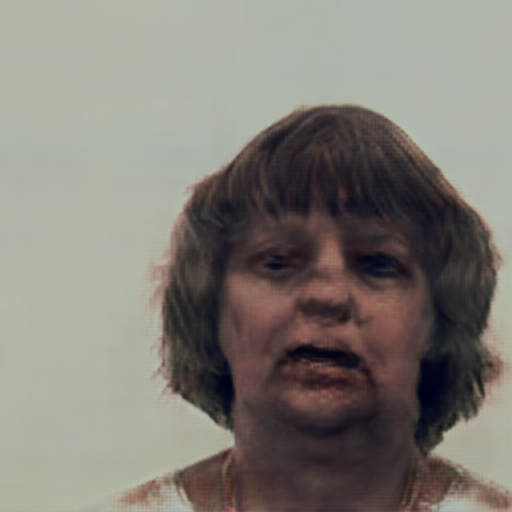}&
                \includegraphics[width=0.13\textwidth]{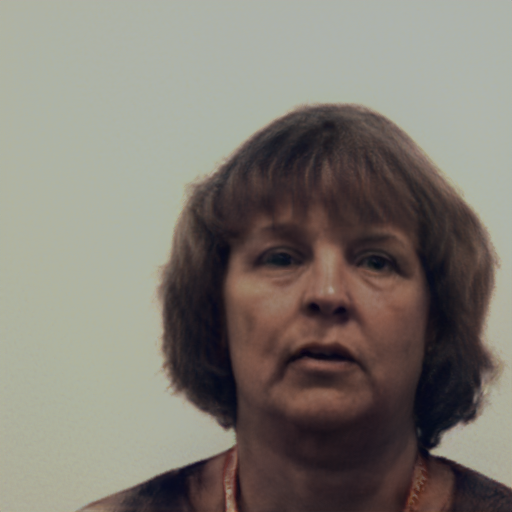}
                \tabularnewline
                GT/TH & pixel2pixel~\cite{isola2017image} & HiFaceGAN~\cite{yang2020hifacegan} & GANVFS~\cite{zhang2019synthesis}&SAGAN~\cite{di2019polarimetric}&AxialGAN~\cite{immidisetti2021simultaneous}&\textbf{VPGAN}
            \end{tabular}
            }
            \vspace{-0.1cm}
            \caption{Visual comparison on the ARL-VTF dataset.}
            \vspace{-0.3cm}
            \label{fig:fig4}
        \end{figure*}
